# Supplementary material for: SMart: A Multi-source Multi-phase Time Series Representation Transfer Framework
Source: arXiv:2609.02203 source file (2026-09-02)
Supplement: Supplementary file 1 [file appendix.tex]

\clearpage
\section{Hyper-parameter Sensitivity Test of SMart}

In this section, we test the sensitivity of four main hyper-parameters: i) the number of layers in the encoder $n_{lyr}$; ii) model dimension $d_{enc}$ (i.e., dimension of the representation for each time point) of the encoder; iii) dimension of head embedding $d_{head}$ in the cross attention; and iv) model dimension of source selector $d_{sor}$. An overall good setting of these four parameters is: the number of layers in the encoder is 6, the model dimension of the encoder is 64, the dimension of head embeddings in the source selector is 64, and the model dimension of the source selector is 128. To validate the sensitivity of the model performance to these parameters, we vary the parameters by: i) $n_{lyr}$ as 3, 4, 5, 6, and 7; ii) $d_{enc}$ as 16, 32, 64, 128, and 256; iii) $d_{head}$ as 16, 32, 64, 128, and 256; iv) $d_{sor}$ as 16, 32, 64, 128, and 256. 
Figure~\ref{fig:parametersensitivity} shows the results of parameter sensitivity tests. As shown in Figure~\ref{fig:parametersensitivity} (a), the classification accuracy increases and the average MAE decreases with more layers, while both converging after $n_{lyr}=6$. In Figure~\ref{fig:parametersensitivity} (b), we observe that setting $d_{enc}=64$ achieves slightly higher accuracy for classification but a slightly larger MAE for regression than setting $d_{enc}=128$. To cut down the number of parameters, we believe $d_{enc}=64$ is a better choice. In Figure~\ref{fig:parametersensitivity} (c), we observe that setting $d_{head}$ achieves the second highest accuracy (i.e., 87.84\% v.s. the highest accuracy 87.85\%) and the smallest MAE when $d_{head}$ is 64. Besides, increasing $d_{head}$ from 64 to a larger number (e.g., 128 and 256) will slightly decrease both the accuracy and MAE, which may be due to too many model parameters, making the model hard to train. Finally, from Figure~\ref{fig:parametersensitivity} (d), we observe that the performance of classification and regression converges after the model dimension is 128 or higher. Besides, we observe that when $d_{sor}$ is smaller than 32, the performance is worse, which proves that the model performance is sensitive to the model dimension selected in the source selector and it is necessary to select a large enough $d_{sor}$ (at least 128).


\begin{figure}[!ht]
\centering
\includegraphics[width=3.4in]{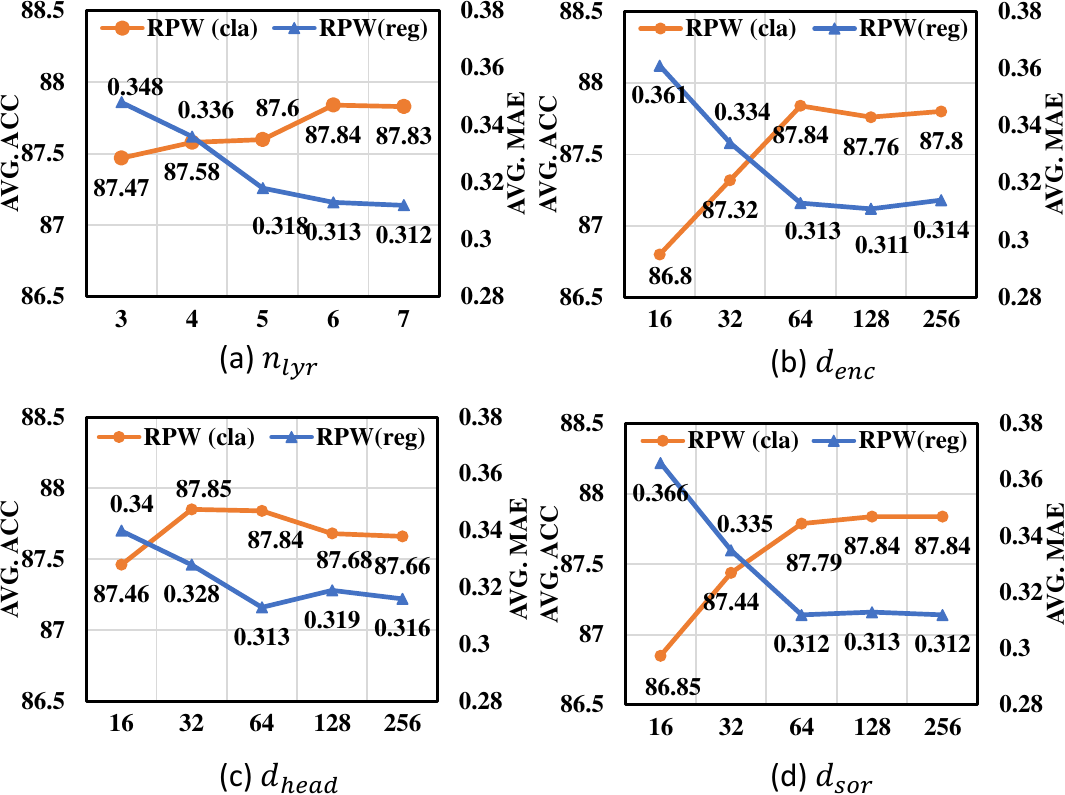}
\caption{Parameter Sensitivity Test}
\label{fig:parametersensitivity}
\end{figure}

\section{Details of Validation and Testing Groups}
In our experiments, we have the following 10 datasets in the validation groups: Computers, RefrigerationDevices, SmallKitchenAppliances, ECG5000, NonInvasiveFetalECGThorax2, MiddlePhalanxTW, SwedishLeaf, CricketZ, InlineSkate, and UWaveGestureLibraryX.

We have the following 10 datasets in the testing groups: WormsTwoClass, ItalyPowerDemand, Lightning2, StarLightCurves, Mallat, Beef, Ham, Meat, InsectWingbeatSound and Strawberry.
The other 65 bake-off datasets are in the training groups.
